# Supplementary material for: Topological Deep Learning: Going Beyond Graph Data
Source: arXiv:2206.00606 source file (2023-05-19)
Supplement: Supplementary file 1 [file appendix_F.tex]

% Section 8
\section{Equivariant higher-order message passing}
\label{sec:equivariantHOMP}

In Section \ref{homp-merge}, we introduce higher-order message passing. Here, we briefly discuss equivariant higher-order message passing over a group $G$.  
This section assumes basic familiarity with group theory.

Let $G$ be a group.  Denote by $\mathrm{GL}(\mathbb{R}^{n})$ the general linear group of degree $n \times n$ invertible matrices.  Assume $G$ acts on the $l$th layer feature space $\mathbb{R}^{d^{(l)}_k}$ via a group representation $\rho^{(l)}_k \colon G \to \mathrm{GL}(\mathbb{R}^{d^{(l)}_k})$. 
 Thus, $G$ acts on data $\mathbf{h}_x^{(l)} \in C^{k}(\CCX, \mathbb{R}^{d^{(l)}}_k)$. Denote by $\rho^{(l)} = \oplus_k \rho^{(l)}_k$ the combined diagonal action on $\oplus_k C^{k}(\CCX, \mathbb{R}^{d^{(l)}}_k)$ across all ranks. We assume $G$ also acts on the messages $m_{x,y}$, $m_k^x$, and $m_x$. In general, these actions may be distinct $\rho^{(l)}_{k}$, i.e., depend on the rank $k$, however, one may also take them to all be equal to $\rho^{(l)}$. Using notation as in Section \ref{homp-merge}, we have the following proposition.

\begin{proposition} If $\alpha_{\mathcal{N}_x}$, $\bigoplus$, $\bigotimes$, and $\beta$ are $G$-equivariant then higher-order message passing over $\CCX$ is $G$-equivariant.  That is, if the function mapping inputs to the hidden layer $l$ is denoted $h^{(l)} = \varphi^{(l)}(h^{(0)})$ then $\varphi^{(l)}$ is equivariant, i.e,
\[
    \rho^{(l)}(g) \varphi^{(l)}( h^{(0)} ) = \varphi^{(l)}(\rho^{(0)}(g) h^{(0)})
\]
for all $g \in G$.
\end{proposition}

\begin{proof}
The proof follows straightforwardly by induction on $l$ and the fact that composition of equivariant functions is equivariant.    
\end{proof}
